# Supplementary material for: Assessing the Impact of Image Dataset Features on Privacy-Preserving Machine Learning
Source: arXiv:2409.01329 source file (2024-12-11)
Supplement: Supplementary file 1 [file appendix_arch.tex]

\begin{table}[H]
    \small
    \begin{center}
    \begin{tabular}{lll}
        \toprule
        \textbf{Layer} & \textbf{Output Shape} & \textbf{\# Parameter} \\\midrule
        RandomFlip              & (32, 32, 3)  & 0 \\
        \midrule
        Conv2D-1 (32, 3x3, 1)   & (32, 32, 32) & 896 \\
        Group Normalization     & (32, 32, 32) & 64 \\
        MaxPooling2D            & (16, 16, 32) & 0 \\
        \midrule
        Conv2D-2 (32, 3x3, 1)   & (16, 16, 32) & 9248 \\
        Group Normalization     & (16, 16, 32) & 64 \\
        MaxPooling2D            & (8, 8, 32)   & 0 \\
        \midrule
        Conv2D-3 (64, 3x3, 1)   & (8, 8, 64)   & 18496 \\
        Group Normalization     & (8, 8, 64)   & 128 \\
        MaxPooling2D            & (4, 4, 64)   & 0 \\
        \midrule
        Flatten                 & (1024)       & 0 \\
        Dense                   & (512)        & 524800 \\
        Group Normalization     & (512)        & 1024 \\
        Dense                   & (10)         & 5130 \\
        \bottomrule
    \end{tabular}
    \end{center}
    \caption{
        Overview of model layers, their output shape and amount of parameters. Each convolution has their number of filters, kernel size, and stride value. We employ a 32-group normalization.
    }
    \label{app-tab:complete_tf_model_parameter_overview}
\end{table}
