# Supplementary material for: Assessing the Impact of Image Dataset Features on Privacy-Preserving Machine Learning
Source: arXiv:2409.01329 source file (2024-12-11)
Supplement: Supplementary file 2 [file appendix_lira.tex]

\begin{figure}[H]
\begin{center}
\includegraphics[width=0.78\textwidth]{figs/lira-online-schema-hists.png}
\end{center}
\caption[Procedure of the LIRA Membership Inference Attack]{
Procedure of the \ac{LiRA} membership inference attack. Shadow models are trained on random samples, half including the query sample $(x,y)$. Confidence outputs are fitted to Gaussian distributions, and a likelihood ratio test determines the sample’s membership probability.}
\label{app-fig:lira-procedure-hists}
\end{figure}
