# Supplementary material for: Assessing the Impact of Image Dataset Features on Privacy-Preserving Machine Learning
Source: arXiv:2409.01329 source file (2024-12-11)
Supplement: Supplementary file 3 [file appendix_res.tex]

\subsection{Class Count Utility Results}\label{app:res_class_count}
    \begin{figure}[H]
        \centering
        \begin{subfigure}[c][][c]{0.328\textwidth}
            \includegraphics[width=\textwidth]{figs/evaluation/non-private-class-count-comparison-2/utility-analysis-combined/run_f1score_comparison_r01234567.png}
            \caption{Non-private ($\varepsilon=\infty$) model.}
        \end{subfigure}
        \hfill
        \begin{subfigure}[c][][c]{0.328\textwidth}
            \includegraphics[width=\textwidth]{figs/evaluation/private-class-count-comparison-2-eps-30/utility-analysis-combined/run_f1score_comparison_r01234567.png}
            \caption{Private ($\varepsilon=30$) model.}
        \end{subfigure}
        \hfill
        \begin{subfigure}[c][][c]{0.328\textwidth}
            \includegraphics[width=\textwidth]{figs/evaluation/private-class-count-comparison-2-eps-1/utility-analysis-combined/run_f1score_comparison_r01234567.png}
            \caption{Private ($\varepsilon=1$) model.}
        \end{subfigure}
        \\
        \begin{subfigure}[c][][c]{0.328\textwidth}
            \includegraphics[width=\textwidth]{figs/evaluation/non-private-class-count-comparison/utility-analysis-combined/run_f1score_comparison_r0123456789.png}
            \caption{Non-private ($\varepsilon=\infty$) model.}
        \end{subfigure}
        \hfill
        \begin{subfigure}[c][][c]{0.328\textwidth}
            \includegraphics[width=\textwidth]{figs/evaluation/private-class-count-comparison-eps-30/utility-analysis-combined/run_f1score_comparison_r0123456789.png}
            \caption{Private ($\varepsilon=30$) model.}
        \end{subfigure}
        \hfill
        \begin{subfigure}[c][][c]{0.328\textwidth}
            \includegraphics[width=\textwidth]{figs/evaluation/private-class-count-comparison-eps-1/utility-analysis-combined/run_f1score_comparison_r0123456789.png}
            \caption{Private ($\varepsilon=1$) model.}
        \end{subfigure}
        \caption{
            F1-scores for non-private and private models on different datasets with modified class counts. Note the scaling of the Y-axes between different privacy budgets.}
        \label{app-fig:class_count_f1_results}
    \end{figure}
    
\subsection{Class Imbalance Utility Results}\label{app:res_class_imbalance}
    \begin{figure}[H]
        \centering
        \begin{subfigure}[c][][c]{0.328\textwidth}
            \includegraphics[width=\textwidth]{figs/evaluation/non-private-imbalance-comparison-l/utility-analysis-combined/run_f1score_comparison_r01234.png}
            \caption{Non-private ($\varepsilon=\infty$) model.}
        \end{subfigure}
        \hfill
        \begin{subfigure}[c][][c]{0.328\textwidth}
            \includegraphics[width=\textwidth]{figs/evaluation/private-imbalance-comparison-l-eps-30/utility-analysis-combined/run_f1score_comparison_r01234.png}
            \caption{Private ($\varepsilon=30$) model.}
        \end{subfigure}
        \hfill
        \begin{subfigure}[c][][c]{0.328\textwidth}
            \includegraphics[width=\textwidth]{figs/evaluation/private-imbalance-comparison-l-eps-1/utility-analysis-combined/run_f1score_comparison_r01234.png}
            \caption{Private ($\varepsilon=1$) model.}
        \end{subfigure}
        \\
        \begin{subfigure}[c][][c]{0.328\textwidth}
            \includegraphics[width=\textwidth]{figs/evaluation/non-private-imbalance-comparison-n/utility-analysis-combined/run_f1score_comparison_r01234.png}
            \caption{Non-private ($\varepsilon=\infty$) model.}
        \end{subfigure}
        \hfill
        \begin{subfigure}[c][][c]{0.328\textwidth}
            \includegraphics[width=\textwidth]{figs/evaluation/private-imbalance-comparison-n-eps-30/utility-analysis-combined/run_f1score_comparison_r01234.png}
            \caption{Private ($\varepsilon=30$) model.}
        \end{subfigure}
        \hfill
        \begin{subfigure}[c][][c]{0.328\textwidth}
            \includegraphics[width=\textwidth]{figs/evaluation/private-imbalance-comparison-n-eps-1/utility-analysis-combined/run_f1score_comparison_r01234.png}
            \caption{Private ($\varepsilon=1$) model.}
        \end{subfigure}
        \caption{F1-scores for non-private and private models on different datasets with modified class imbalance and in linear mode (top) or normal mode (bottom). Note the scaling of the Y-axes between different privacy budgets.}
        \label{app-fig:class_imbalance_f1_results}
    \end{figure}
